# Supplementary material for: Recency-Weighted Temporally-Segmented Ensemble for Time-Series Modeling
Source: arXiv:2403.02150 ancillary file (2024-03-04)
Supplement: Supplementary file 1 [file ReWTS_supplementary_final.pdf]

# Recency-Weighted Temporally-Segmented Ensemble for Time-Series Modeling

## Multi-step Forecasting in Process Industries

Supplementary File

Pål Vegard Johnsen[1*], Eivind Bøhn[1], Sølve Eidnes[1], Filippo Remonato[1], and Signe Riemer-Sørensen[1]

[1]SINTEF Digital, Oslo, Norway
[*]Corresponding author: pal.johnsen@sintef.no

March 4, 2024

# 1 ReWTS weight fitting derivation

In this section we will provide the ReWTS weight fitting procedure, the optimization problem and the corresponding closed-form solution.

We let $\mathcal{M}_k$ denote the set of fitted forecasting models at time $t_k$. Further, the vector $\mathbf{y}_{(k+1):(k+h)}$ yields the target values from time $t_{k+1}$ to $t_{k+h}$, and the matrix $M_h(X_{:k}, \mathbf{y}_{:k})$ of dimension $h\times \mid \mathcal{M}_k \mid$ includes the next $h$ predictions for each model at time $t_k$.

Assume we are at the present time point $t_n$ with a look-back data of length $l_b$ given the most recent data points going back $l_b$ time steps back in time. Then, we want to find the weights, $\mathbf{w}(t_n)$, that satisfies

$$\arg\min_{\mathbf{w}(t_n)} \sum_{k=n-l_b}^{n-h} \Big(\mathbf{y}_{(k+1):(k+h)} - M_h\left(X_{:k}, \mathbf{y}_{:k}\right)\mathbf{w}(t_n)\Big)^T \Big(\mathbf{y}_{(k+1):(k+h)} - M_h\left(X_{:k}, \mathbf{y}_{:k}\right)\mathbf{w}(t_n)\Big) \tag{1}$$

$$\text{s.t.} \quad \mathbf{w}(t_n) \geq 0$$
$$\mathbf{1}^T \cdot \mathbf{w}(t_n) = 1.$$

We can rewrite the optimization problem:

$$
\begin{aligned}
&\arg\min_{\mathbf{w}(t_n)} \sum_{k=n-l_b}^{n-h} \Big(\mathbf{y}_{(k+1):(k+h)} - M_h\left(X_{:k}, \mathbf{y}_{:k}\right) \mathbf{w}(t_n)\Big)^T \Big(\mathbf{y}_{(k+1):(k+h)} - M_h\left(X_{:k}, \mathbf{y}_{:k}\right) \mathbf{w}(t_n)\Big) \\
&= \arg\min_{\mathbf{w}(t_n)} \sum_{k=n-l_b}^{n-h} \left(\mathbf{y}_{(k+1):(k+h)}\right)^T \left(\mathbf{y}_{(k+1):(k+h)}\right) + \mathbf{w}(t_n)^T M_h(X_{:k}, \mathbf{y}_{:k})^T M_h(X_{:k}, \mathbf{y}_{:k}) \mathbf{w}(t_n) \\
&- 2\mathbf{y}_{(k+1):(k+h)}^T M_h(X_{:k}, \mathbf{y}_{:k}) \mathbf{w}(t_n) \\
&= \arg\min_{\mathbf{w}(t_n)} \frac{1}{2} \mathbf{w}(t_n)^T \left( \sum_{k=n-l_b}^{n-h} M_h(X_{:k}, \mathbf{y}_{:k})^T M_h(X_{:k}, \mathbf{y}_{:k}) \right) \mathbf{w}(t_n) \qquad (2) \\
&- \left( \sum_{k=n-l_b}^{n-h} M_h(X_{:k}, \mathbf{y}_{:k})^T \mathbf{y}_{(k+1):(k+h)} \right)^T \mathbf{w}(t_n) \\
\\
&\text{s.t.} \quad \mathbf{w}(t_n) \geq 0 \\
&\qquad\ \ \mathbf{1}^T \cdot \mathbf{w}(t_n) = 1.
\end{aligned}
$$

Let $Q = \sum_{k=n-l_b}^{n-h} M_h(X_{:k}, \mathbf{y}_{:k})^T M_h(X_{:k}, \mathbf{y}_{:k})$, a matrix of dimension $\mid \mathcal{M}_k \mid \times \mid \mathcal{M}_k \mid$, and let $p = \sum_{k=t-L}^{t-h} M_h(X_{:k}, \mathbf{y}_{:k})^T \mathbf{y}_{(k+1):(k+h)}$, a vector of size $\mid \mathcal{M}_k \mid$, and plug in these variables into the optimization problem (2). The matrix $Q$ is symmetric as it is a sum of symmetric matrices. This structure of the optimization problem, with the fact that $Q$ is symmetric, makes it a *quadratic programming* (QP) optimization problem. Additionally, the matrix $Q$ is positive semidefinite, because it is a sum of positive semidefinite matrices ($M^T M$ positive semidefinite for any matrix $M$ of dimension $m \times n$). In this case, we say that we have a *convex* QP problem for which there exist efficient solvers [1]. The software used in this work in the CVXOPT package in python [2].

Both the matrix $Q$ and the vector $p$ is a sum of multiple matrices or vectors respectively, and the number of summands increases proportionally with the look-back length. Depending on the scaling of the target $y$, some elements in the matrix $Q$ and vector $p$ might therefore become very big in magnitude. This may yield numerical instabilities in the QP-solver, and occasionally non-convergence and ultimately errors. These instabilities can also happen for elements that are very small in magnitude. One simple way to circumvent these potential issues is to rescale the matrix $Q$ and vector $p$ in cases where the element with the maximum value is very small, $\max(Q_{ij}, p_j) < \epsilon$, given by some predefined threshold $\epsilon$, or the element with the maximum value is very large, $\max(Q_{ij}, p_j) > L$, given by some predefined threshold $L$. In these cases, $Q$ and $p$ in (2) can be rescaled to $Q' = Q/\epsilon, p' = p/\epsilon$ or $Q' = Q/L, p' = p/L$ respectively. Swapping $Q, p$ with $Q', p'$ in the optimization problem (2) will not alter the solution, $\mathbf{w}(t_n)$, of the original QP-problem.

# 2 ReWTS weight fitting with $h = 1$

**Algorithm 3** The one-step weight fitting with forecasting horizon $h$ - ReWTS ensemble model

▷ Given forecast horizon, $h$, look-back length , $l_b$, chunk length, $l_c$, stride $s$ and present time point $t_n$ with $n/l_c$ an integer.
▷ Assign $C = n/l_c$, the number of available chunks
▷ Assign $v = n$
▷ Given all previously trained models, $\mathcal{M}_v = \{M_1, ..., M_C\}$ from the $C$ previous chunks
**repeat**
  **while** $v \leq (C+1) \cdot l_c$ **do**
    ▷ Collect look-back data $(X_{(v-l_b):v}, \mathbf{y}_{(v-l_b):v})$
    ▷ Calculate the weights $\hat{\mathbf{w}}(t_v)$ according to optimization problem (2) with $h = 1$ given chunk models in $\mathcal{M}_v$
    **for** $j = 1 : h$ **do**
      **if** $j = 1$ **then**
        ▷ Compute one-step ahead forecast at time $t_{v+1}$ for each chunk model, and save in $1 \times |\mathcal{M}_v|$ matrix $M_1(X_{:v}, \mathbf{y}_{:v})$
        ▷ Compute final forecast at time point $t_{v+1}$ by ReWTS ensemble given by $\hat{y}_{v+1} = M_1(X_{:v}, \mathbf{y}_{:v})\hat{\mathbf{w}}(t_v)$
      **else if** $j > 1$ **then**
        ▷ Compute one-step ahead forecast at time $t_{v+j}$ for each chunk model by using the previous predictions $\hat{\mathbf{y}}_{v+k}$ for $k = 1, \ldots, j-1$, and save in $1 \times |\mathcal{M}_v|$ matrix $M_1(X_{:(v+j-1)}, \hat{\mathbf{y}}_{:(v+j-1)})$, with $\hat{\mathbf{y}}_{:(v+j-1)}$ including all known previous values of the target as well as the most recent predictions of the target
        ▷ Compute final forecast by ReWTS ensemble at time $t_{v+j}$ given by $\hat{y}_{v+j} = M_1(X_{:(v+j-1)}, \hat{\mathbf{y}}_{:(v+j-1)})\hat{\mathbf{w}}(t_v)$
      **end if**
    **end for**
    ▷ $v = v + s$
  **end while**
  ▷ Collect all data from new chunk number $C + 1$ between time points $t_{C \cdot l_c}$ and $t_{(C+1) \cdot l_c}$
  ▷ Train new chunk model $M_{C+1}$ from chunk $C + 1$ and update $\mathcal{M}_v$
  ▷ $C = C + 1$
**until** Collection of new data stops

In Algorithm 1 in the main article, the forecasting procedure for the ReTWS ensemble model is described in detail. In this procedure, there is a match between the parameter $h$ in Algorithm 1 used during the weight fitting procedure, and the desired forecast horizon of the ReTWS ensemble model during forecasting. This is reasonable, but not a requirement. One alternative for one-step ahead autoregressive models is to set $h = 1$ in the QP optimization problem (2), which in practice means that we search for the weights that minimize the average MSE of the one step ahead predictions in the look-back data set. The fitted weights can afterwards be used recursively to provide the desired forecast horizon at prediction time. The forecasting procedure in this case is given in Algorithm 3.

# 3 Results on drinking water treatment plant

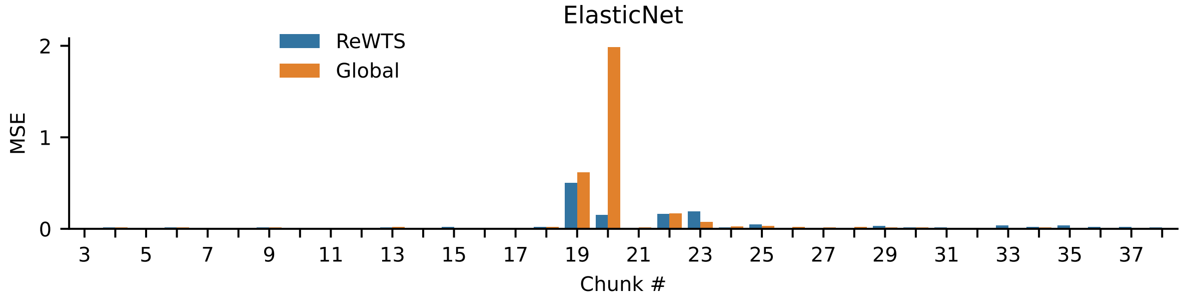


(a) Elastic net model

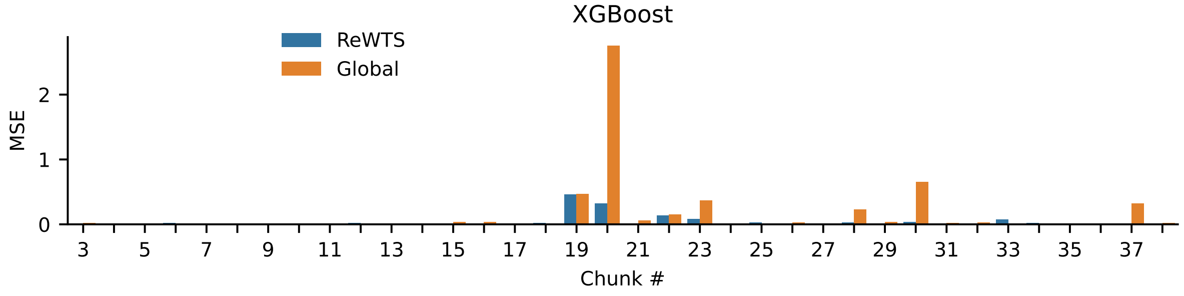


(b) XGBoost model

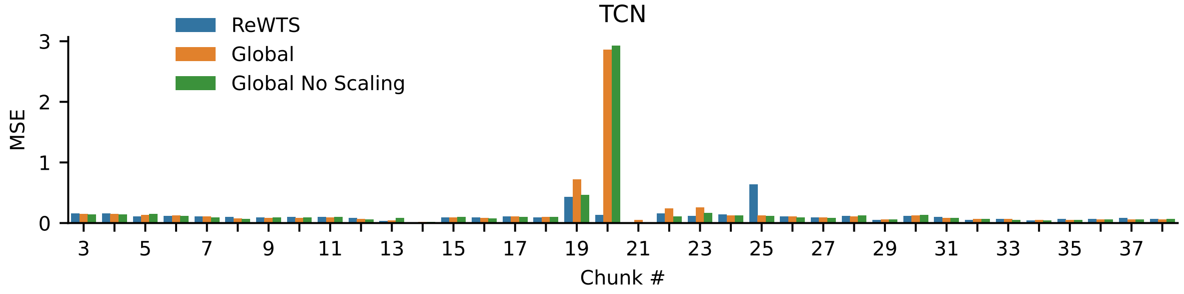


(c) TCN model

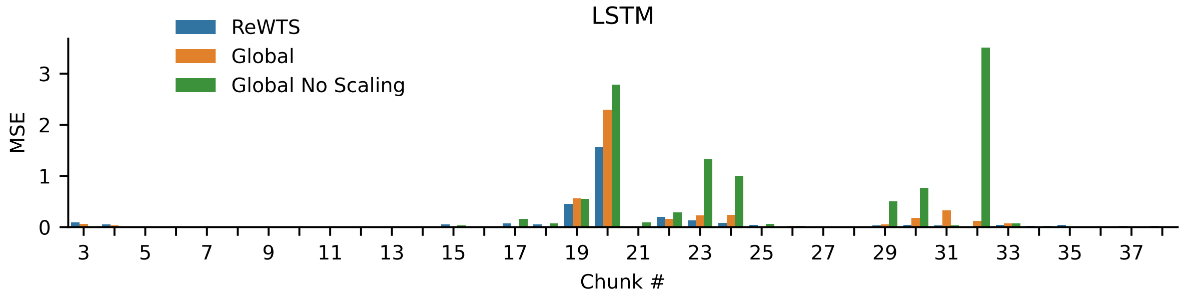


(d) Vanilla LSTM model

Figure 1: Comparing the ReWTS ensemble model with the corresponding global model for the wastewater plant data for the model architectures elastic net, XGBoost, TCN and LSTM. The TCN and LSTM model were upscaled for each new chunk such as to match the total number of trainable parameters by the ReWTS ensemble model. For comparison, a global model without upscaling (Global No Scaling) is also presented.

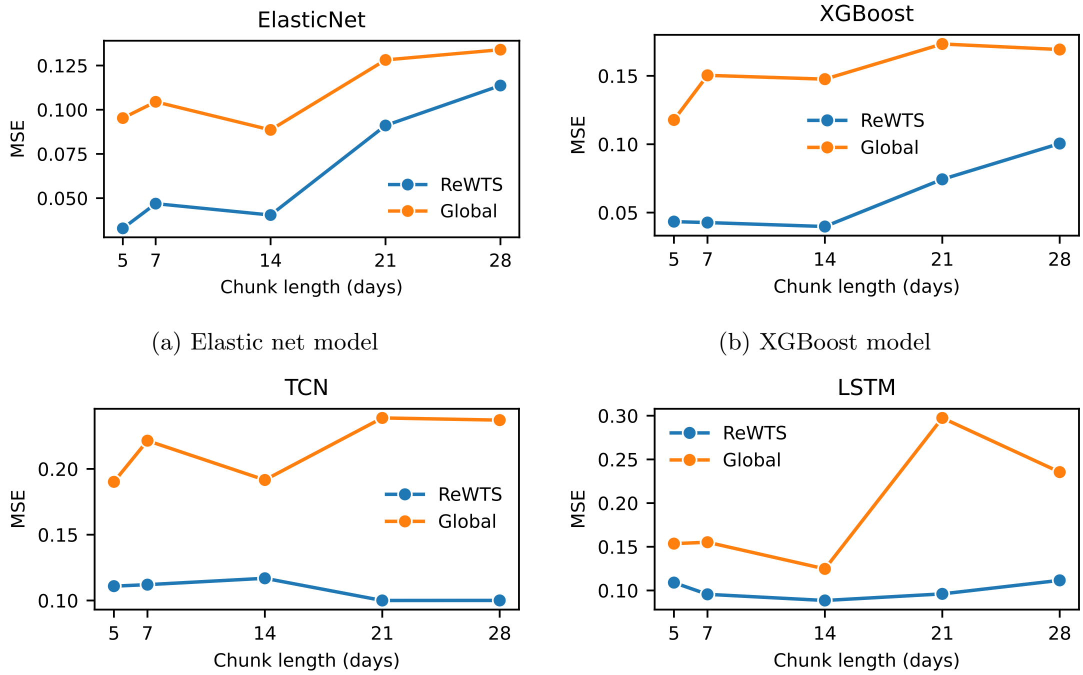


(a) Elastic net model (b) XGBoost model

(c) TCN model (d) Vanilla LSTM model

Figure 2: The average MSE, for different model architectures, of the ReWTS ensemble model for varying chunk length (with constant look-back length of 300 data points). The results are compared with the corresponding global model.

Figure 1 shows the chunk-by-chunk MSE result for the ReWTS ensemble model and the global model, for all model architectures, on the data from the water treatment plant with chunk length of 2016 time points (corresponding to two weeks of data), and a look-back data length of 300 time points (corresponding to two days of data). The story is the same across all the model architectures investigated in this work, namely that the ReWTS ensemble outperforms the global model, with or without up-scaling of trainable parameters.

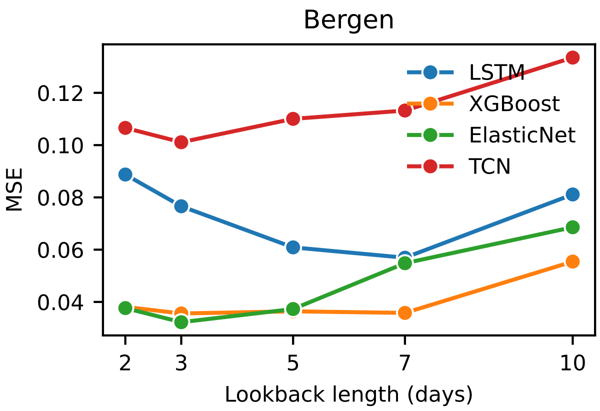


Figure 3: The average MSE, for different model architectures, of the ReWTS ensemble model for varying look-back length (with constant chunk length equal to two weeks of data). Results are given for the wastewater treatment data.

Figure 2 shows the average MSE of the ReWTS ensemble model for varying chunk lengths when

applied on the drinking water treatment data set. Figure 3 shows the average MSE for varying look-back lengths. Mostly, the trend is the same for both the wastewater and drinking water data sets: Within the observed range, smaller chunk and look-back lengths yield smaller average MSE. Exceptions are the TCN model when varying chunk length, and the LSTM model when varying the look-back length.

# 4 Forecast on the simulation data

Below are the forecasts for all chunks, from the ReWTS ensemble model and the global model for the simulation data explained in Section 6.1 in the main article.

## 4.1 Training Set

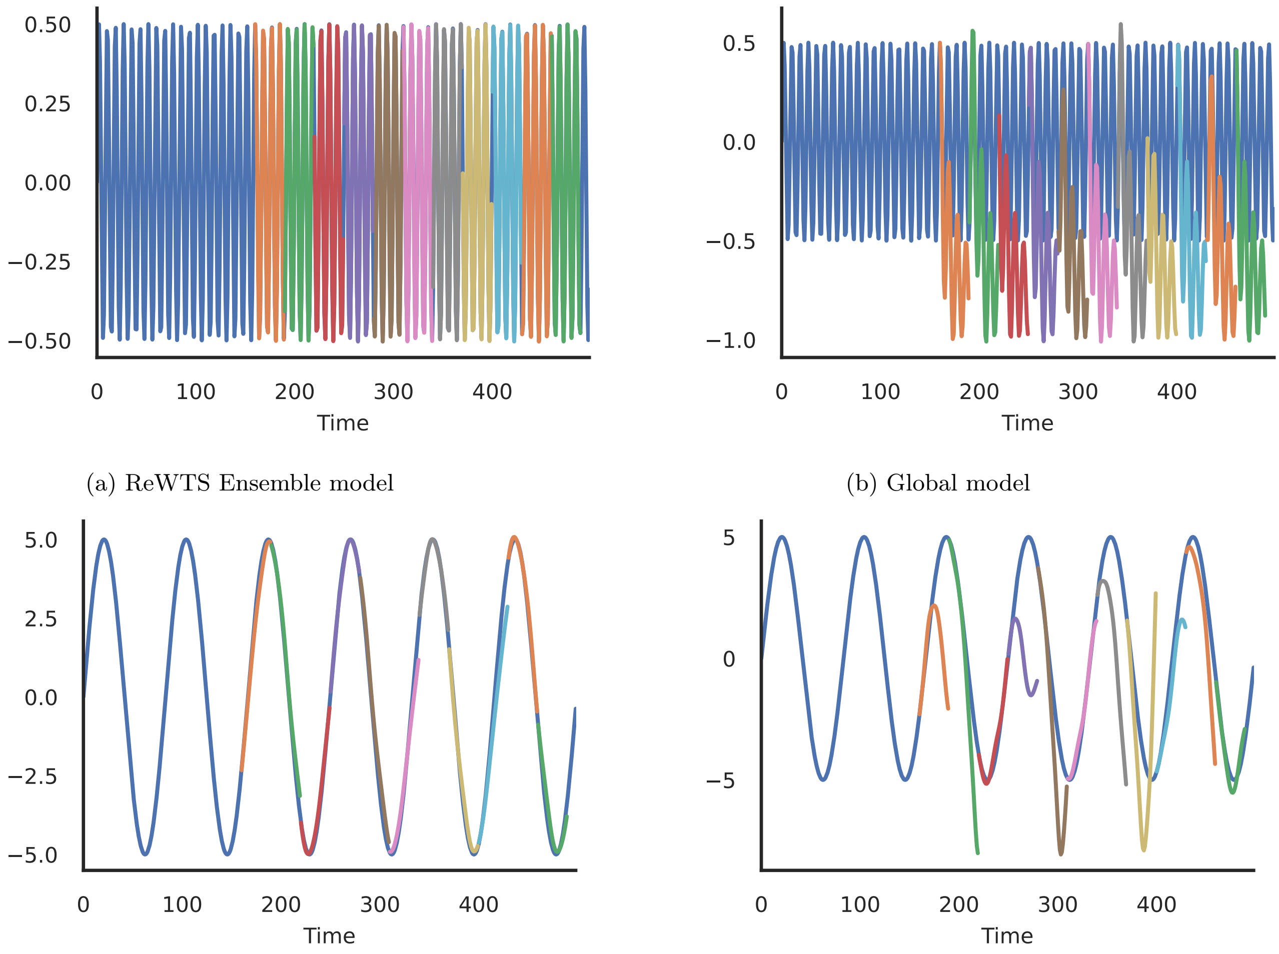


(a) ReWTS Ensemble model

(b) Global model

(c) ReWTS Ensemble model

(d) Global model

Figure 4: Training set, chunks 1, 2

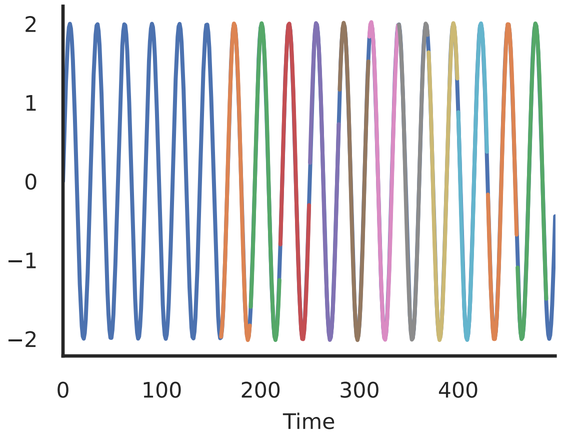


(a) ReWTS Ensemble model

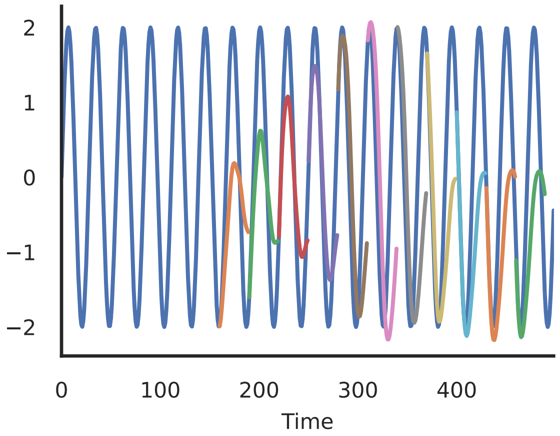


(b) Global model

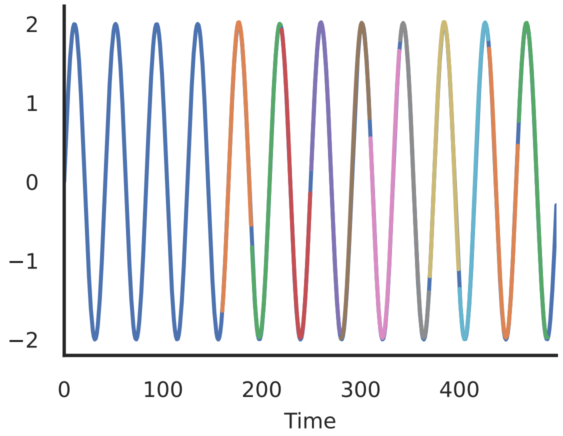


(c) ReWTS Ensemble model

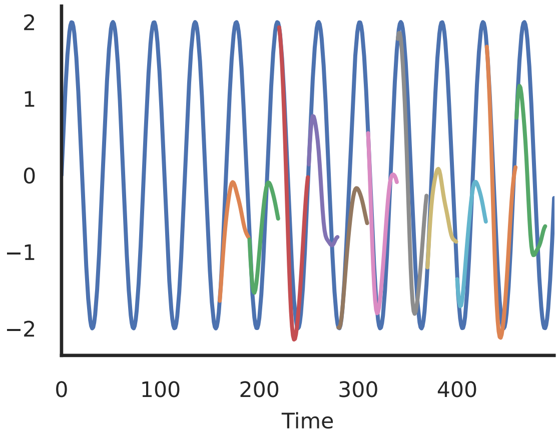


(d) Global model

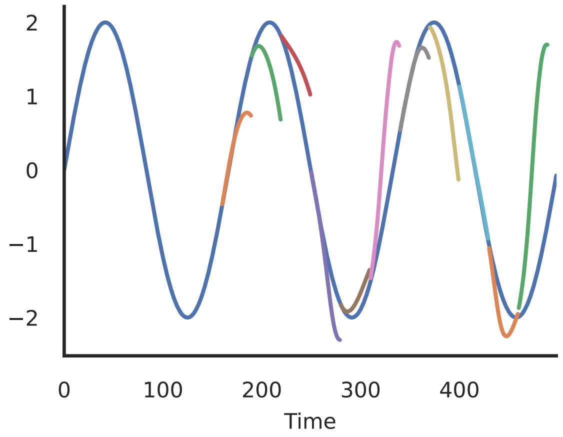


(e) ReWTS Ensemble model

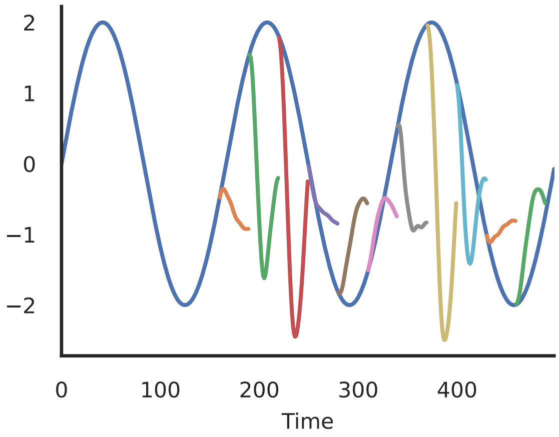


(f) Global model

Figure 5: Training set, chunks 3, 4 and 5

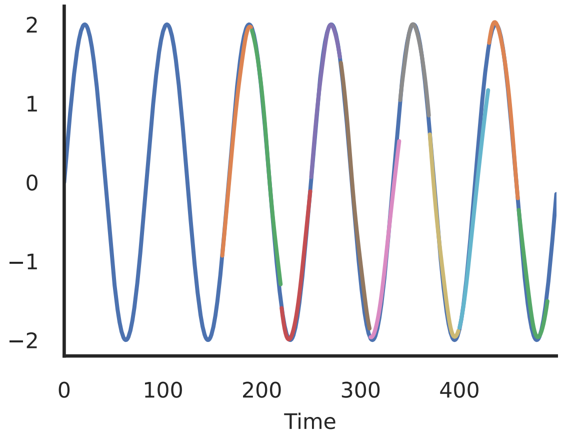


(a) ReWTS Ensemble model

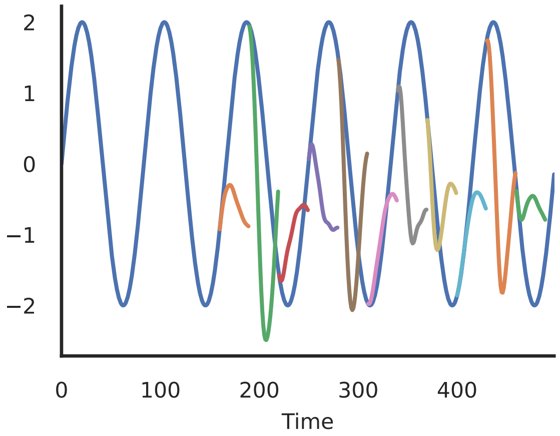


(b) Global model

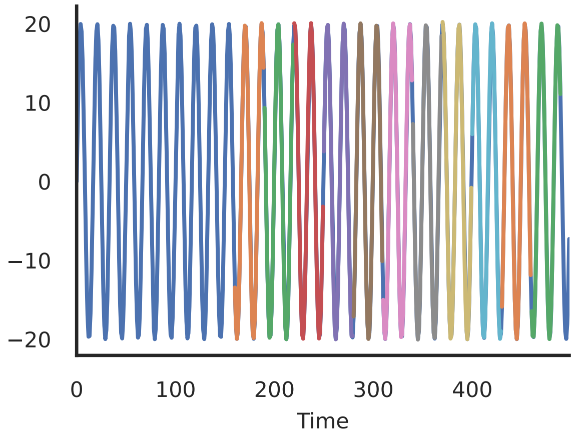


(c) ReWTS Ensemble model

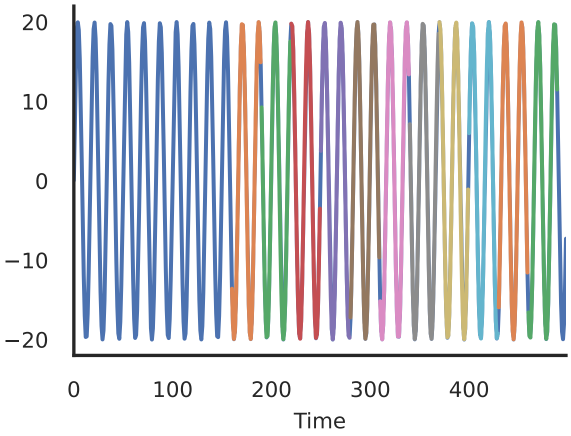


(d) Global model

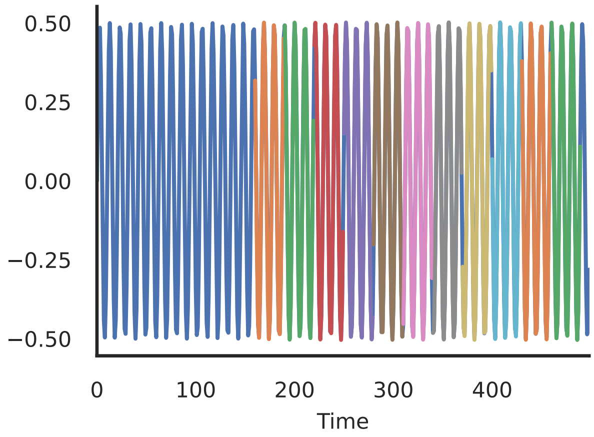


(e) ReWTS Ensemble model

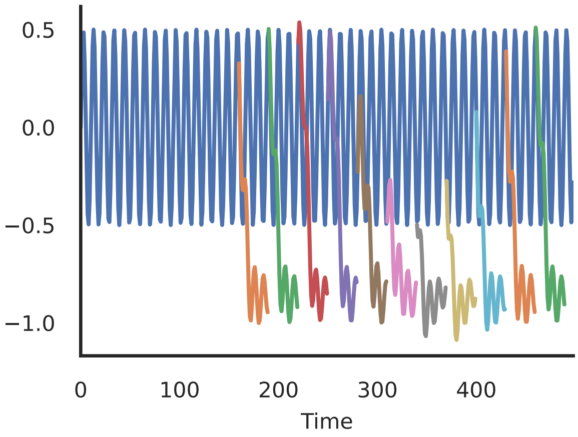


(f) Global model

Figure 6: Training set, chunks 6, 7 and 8

## 4.2 Test Set

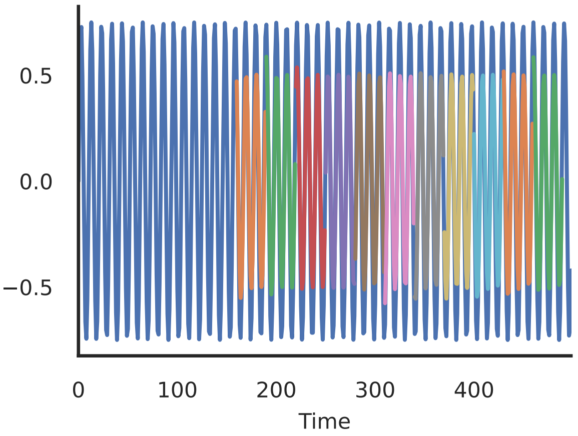


(a) ReWTS Ensemble model

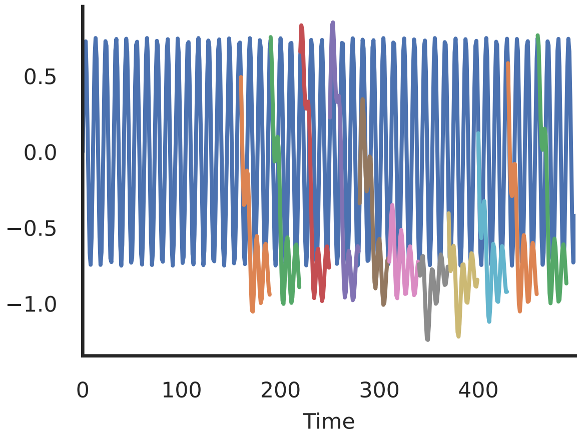


(b) Global model

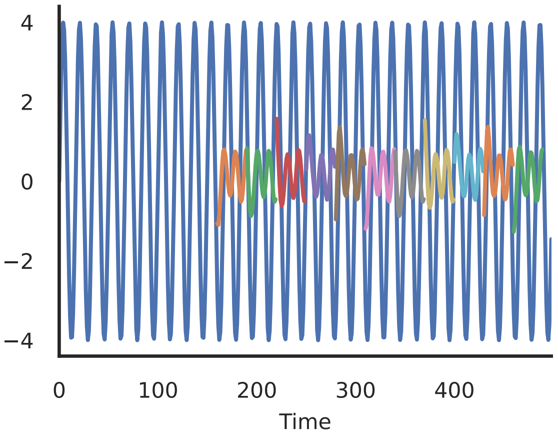


(c) ReWTS Ensemble model

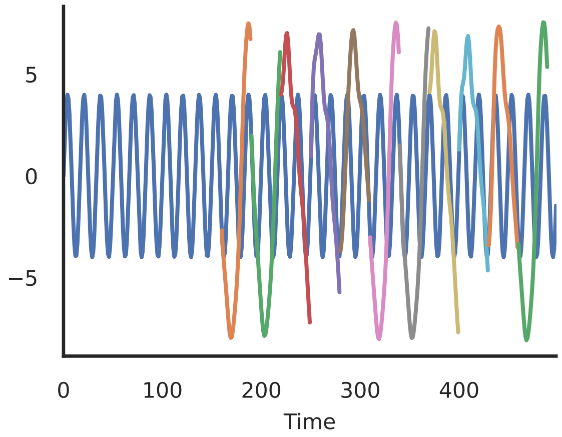


(d) Global model

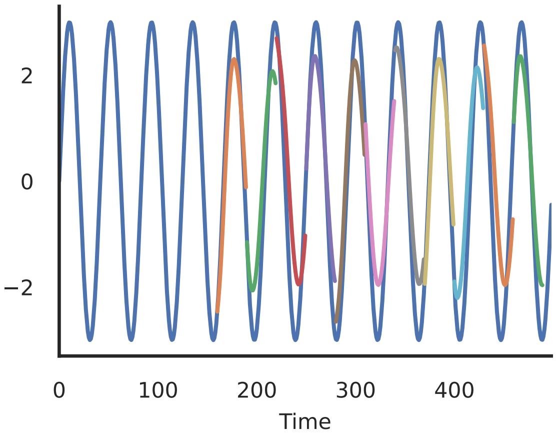


(e) ReWTS Ensemble model

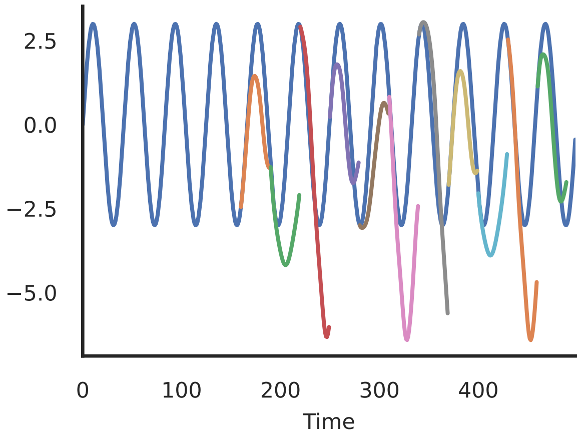


(f) Global model

Figure 7: Test set, chunks 1, 2 and 3

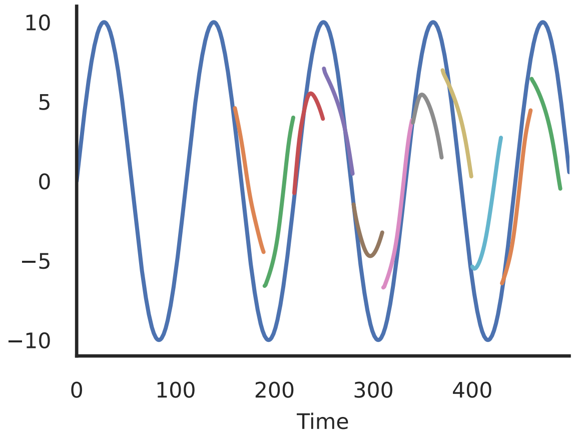


(a) ReWTS Ensemble model

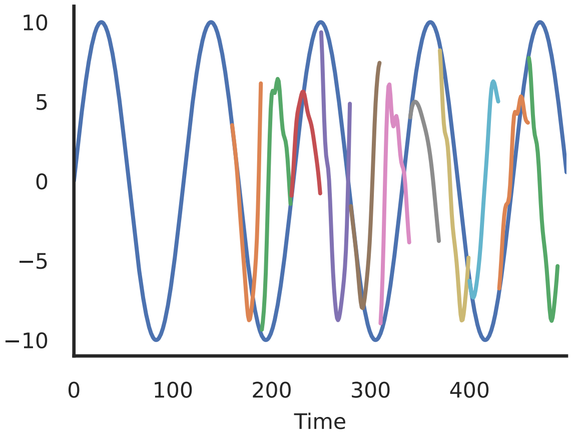


(b) Global model

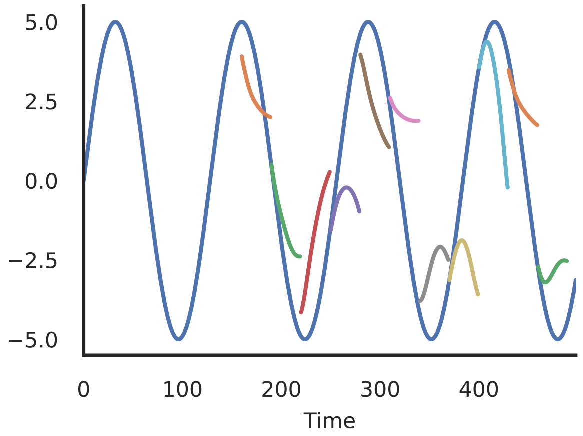


(c) ReWTS Ensemble model

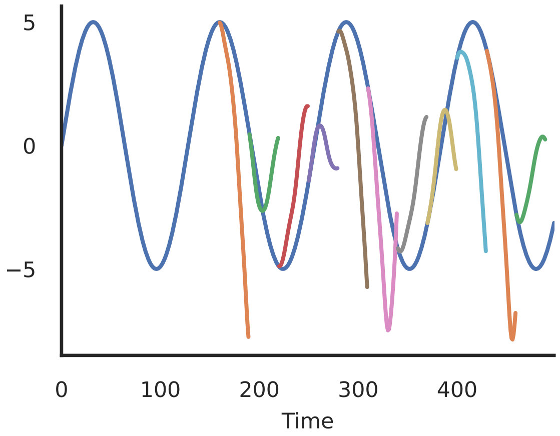


(d) Global model

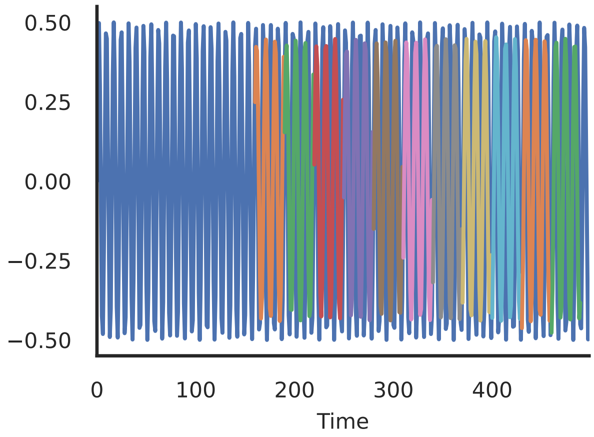


(e) ReWTS Ensemble model

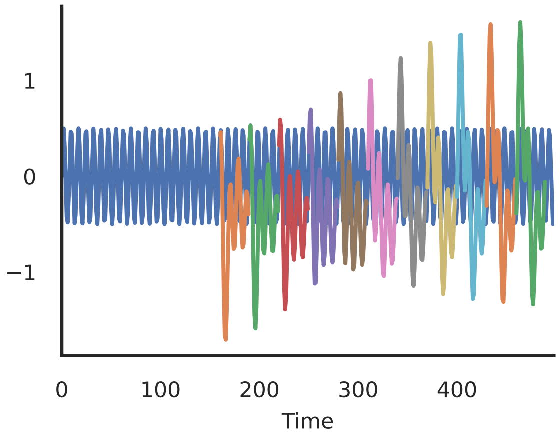


(f) Global model

Figure 8: Test set, chunks 4, 5 and 6

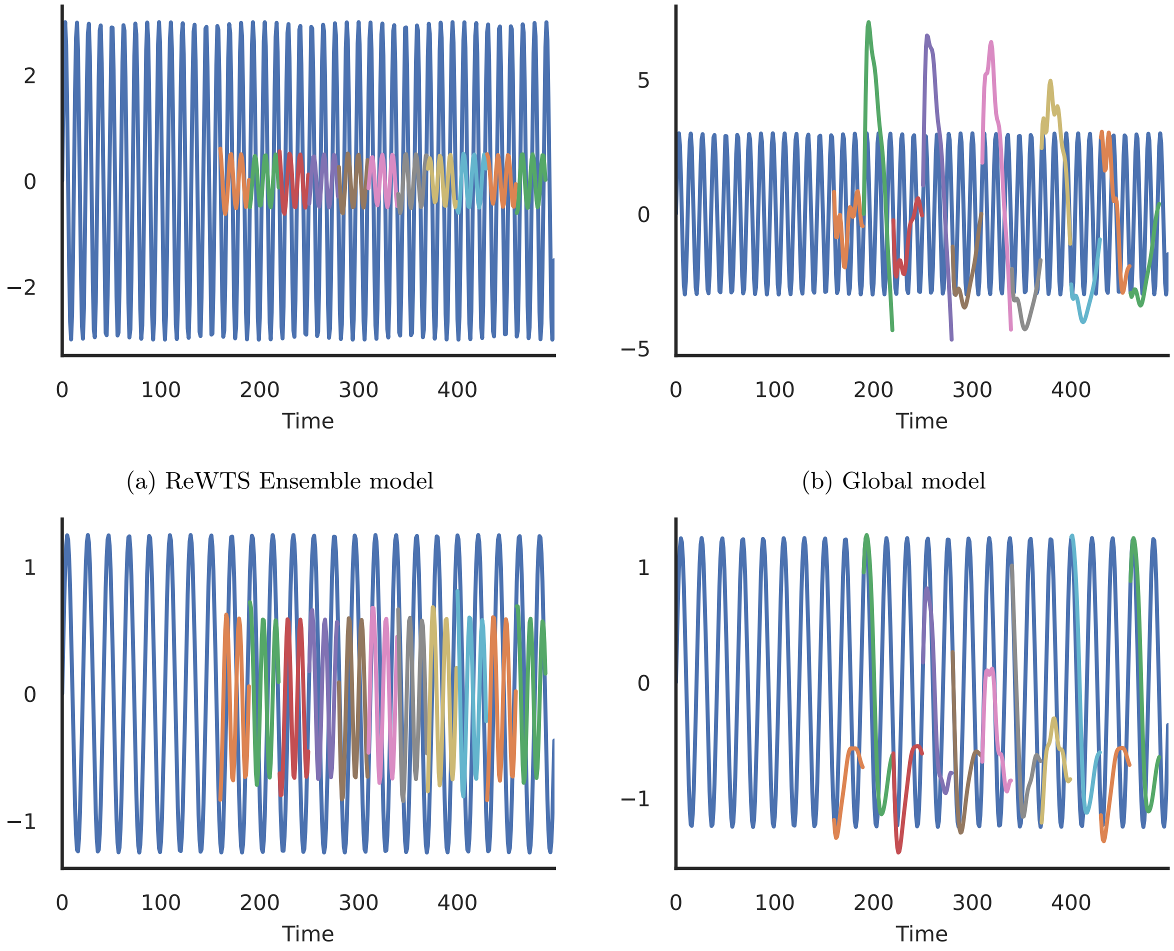


(a) ReWTS Ensemble model

(b) Global model

(c) ReWTS Ensemble model

(d) Global model

Figure 9: Test set, chunks 7 and 8

# References

[1] J. Nocedal and S. J. Wright, *Numerical Optimization*, 2nd. New York, NY: Springer, 2006, ch. 16, ISBN: 0-387-30303-0.

[2] M. S. Andersen, J. Dahl, and L. Vandenberghe, *CVXOPT: A python package for convex optimization, version 1.1.6*, `http://cvxopt.org`, Available at `http://cvxopt.org`, 2013.
